# Supplementary material for: Large-System Analysis of Massive MIMO with Optimal M-MMSE Processing
Source: arXiv:1903.09783 source file (2019-06-25)
Supplement: Supplementary file 1 [file appendices.tex]

\newpage
\begin{figure*}
 \begin{align}
 {\bf T}_{j}^{\star} &= \left(\left(\frac{1}{M}\left(\frac{\frac{MK}{P} \nu}{1+\mu^\star} + \frac{\frac{MK}{P}\nu\alpha(L-1)}{1+\alpha\mu^\star}\right)+\frac{1}{M}\frac{MK}{P} (1-\nu)\overline L\right){\bf A}{\bf A}^{\Htran} + \frac{1}{M{\rho}}{\bf I}_M\right)^{-1}\\&=\left(\frac{K}{P}\underbrace{\left(\frac{\nu}{1+\mu^\star} + \frac{\nu\alpha(L-1)}{1+\alpha\mu^\star}+ (1-\nu)\overline L\right)}_{\eta^\star\overline L}{\bf A}{\bf A}^{\Htran}+ \frac{1}{M{\rho}}{\bf I}_M\right)^{-1}
  \end{align}
  \hrule
  \begin{align}\label{boundT}
\frac{M}{KL}\frac{1}{\underbrace{\max_{jli}||\vect{\Phi}_{jlli}||_2 + \max_{jli}||\vect{R}_{jli} - \vect{\Phi}_{jlli}||_2 + \frac{1}{KL}}_{\varsigma}}{\bf I}_M \preceq {\bf T}_j^{\star} \preceq \frac{M}{KL}\frac{1}{\underbrace{\min_{jli} \lambda_{\min}(\vect{R}_{jli} - \vect{\Phi}_{jlli})}_{\eta}}{\bf I}_M
\end{align}
\hrule
  \end{figure*}
\section*{Appendix B}
Under Assumption~\ref{assumption_3}, the matrix ${\bf T}_j^{\star}$ can be bounded as in \eqref{boundT} at top of the page. Hence, from \eqref{sigma_jk_1} we have that 
%\begin{align}\notag
%\big[\vect{B}_{jk} \big]_{j,j} = \frac{1}{M}\tr \left(  \vect{\Phi}_{jjjk} {\bf T}_{j}^{\star}\right) &\mathop\le^{{(a)}} ||\vect{\Phi}_{jjjk}||_2\frac{1}{M}\tr \left(  {\bf T}_{j}^{\star}\right)\\&\mathop\le^{{(b)}}\frac{M}{KL}\frac{||\vect{\Phi}_{jjjk}||_2}{\eta}
%\end{align}
%where $(a)$ follows from $\tr \left( \vect{A} \vect{B}\right) \le \| \vect{A} \|_2\tr \left( \vect{B}\right)$ and $(b)$ comes from the right-hand-side of \eqref{boundT}. Also, we have that 
%\begin{align}
%\big[\vect{B}_{jk} \big]_{j,j} = \frac{1}{M}\tr \left(  \vect{\Phi}_{jjjk} {\bf T}_{j}^{\star}\right) &\mathop\ge^{{(a)}} \frac{M}{KL} \frac{1}{\varsigma}\frac{1}{M}\tr \left(  \vect{\Phi}_{jjjk} \right)
%\end{align}
%where $(a)$ comes from the left-hand-side of \eqref{boundT}. Putting these results together yields
\begin{align}\label{B.3}
 &\!\!\!\!\!\!\frac{M}{KL} \frac{1}{\varsigma}\frac{1}{M}\tr \left(  \vect{\Phi}_{jllk} \right) \le \big[\vect{B}_{jk} \big]_{l,l}\le \frac{M}{KL}\frac{1}{\eta}\frac{1}{M}\tr \left(  \vect{\Phi}_{jllk} \right)
% \\
%  &\!\!\!\!\!\!\frac{M}{KL} \frac{1}{\varsigma}\frac{1}{M}\tr \left(  \vect{\Phi}_{jl'lk} \right) \le \big[\vect{B}_{jk} \big]_{l,l'}\le \frac{M}{KL}\frac{1}{\eta}\frac{1}{M}\tr \left( \vect{\Phi}_{jl'lk} \right)\label{B.3.1}
\end{align}
which implies that the first term in \eqref{eq:general result_1} is of order $\Omega(M/K)$. For the second term in \eqref{eq:general result_1}, we notice that
\begin{align}\label{B.4}
 \frac{1}{L-1} \tr \left(  \vect{B}_{jk}^{[jj]} \right) \vect{I}_{L-1}\preceq \vect{B}_{jk}^{[jj]} \preceq \tr \left(  \vect{B}_{jk}^{[jj]} \right) \vect{I}_{L-1}.
\end{align}
By using ${\bf x}^{\Htran}\vect{A}{\bf x}^{\Htran} \le {\bf x}^{\Htran}\vect{C}{\bf x}^{\Htran}$ if $\vect{C}-\vect{A} \succeq \vect{0} $, we have that
\begin{align}\notag
{\big(\vect{b}_{jk}^{[j]}\big)}^{\Htran}&\left(  {\bf I}_{L-1}+ \vect{B}_{jk}^{[jj]}\right)^{-1}\!\!\!\vect{b}_{jk}^{[j]} \mathop\ge^{{(a)}} \frac{\sum\limits_{l=1}^{L-1}{(\big[\vect{B}_{jk}^{[jj]}\big]_{ll}})^2}{1 + \tr \left(  \vect{B}_{jk}^{[jj]} \right) } \\&\mathop\ge^{{(b)}}\frac{(\frac{M}{KL})^2 \frac{1}{\varsigma^2} \sum\limits_{l=1,l\ne j}^{L} \big(\frac{1}{M}\tr \left(  \vect{\Phi}_{jllk} \right)\big)^2}{1 + \frac{M}{KL} \frac{1}{\eta} \sum\limits_{l=1,l\ne j}^{L} \frac{1}{M}\tr\left(  \vect{\Phi}_{jllk} \right)}
\end{align}
where $(a)$ and $(b)$ follow from the right-hand-sides of \eqref{B.4} and \eqref{B.3}, respectively. Similarly, we have that 
\begin{align}\notag
{\big(\vect{b}_{jk}^{[j]}\big)}^{\Htran}&\left(  {\bf I}_{L-1}+ \vect{B}_{jk}^{[jj]}\right)^{-1}\!\!\!\vect{b}_{jk}^{[j]} \mathop\le^{{(a)}} \frac{\sum\limits_{l=1}^{L-1}{(\big[\vect{B}_{jk}^{[jj]}\big]_{ll}})^2}{1 +  \frac{1}{L-1}\tr \left(  \vect{B}_{jk}^{[jj]} \right) } \\&\mathop\le^{{(b)}}\frac{(\frac{M}{KL})^2 \frac{1}{\varsigma^2} \sum\limits_{l=1,l\ne j}^{L} \big(\frac{1}{M}\tr \left(  \vect{\Phi}_{jllk} \right)\big)^2}{1 + \frac{M}{KL}  \frac{1}{L-1}\frac{1}{\eta} \sum\limits_{l=1,l\ne j}^{L} \frac{1}{M}\tr\left(  \vect{\Phi}_{jllk} \right)}.
\end{align}
%Therefore, it can be lower bounded as follows:
%\begin{align}\notag
%{\big(\vect{b}_{jk}^{[j]}\big)}^{\Htran}&\left(  {\bf I}_{L-1}+ \vect{B}_{jk}^{[jj]}\right)^{-1}\!\!\!\vect{b}_{jk}^{[j]} \\\notag&\mathop\ge^{{(a)}} \frac{\sum\limits_{l=1}^{L-1}{(\big[\vect{B}_{jk}^{[jj]}\big]_{ll}})^2}{1 + \|\vect{B}_{jk}^{[jj]} \|_2} \\&\mathop\ge^{{(b)}}\frac{\sum\limits_{l=1}^{L-1}{(\big[\vect{B}_{jk}^{[jj]}\big]_{ll}})^2}{1 + \frac{M}{KL} \frac{1}{\eta} \sum\limits_{l=1,l\ne j}^{L} \frac{1}{M}\tr\left(  \vect{\Phi}_{jllk} \right)}\\&\mathop\ge^{{(c)}}\frac{(\frac{M}{KL})^2 \frac{1}{\varsigma^2} \sum\limits_{l=1,l\ne j}^{L} \big(\frac{1}{M}\tr \left(  \vect{\Phi}_{jllk} \right)\big)^2}{1 + \frac{M}{KL} \frac{1}{\eta} \sum\limits_{l=1,l\ne j}^{L} \frac{1}{M}\tr\left(  \vect{\Phi}_{jllk} \right)}
%\end{align}
%where $(a)$ follows from $\tr \left( (\vect{I}+\vect{A})^{-1} \vect{B}\right) \ge \frac{1}{1+\| \vect{A} \|_2}\tr \left( \vect{B}\right)$, $(b)$ from the right-hand-side of \eqref{B.4} and \eqref{B.3}, and $(c)$ from the left-hand-side of \eqref{B.3}.

\section*{Appendix C}
If the channel is modelled as in \eqref{corr_model}, then $\vect{Z}_{j} $ and $\vect{\Theta}_{jll'i}$ are diagonal matrices with entries
%\begin{align}\label{cov_model}
%\vect{\Phi}_{jlli} &= \diag\left({\phi}_{jli}(1),\ldots,{\phi}_{jli}(M)\right)\\
%\vect{Z}_{j} &= \diag\left({z}_{j}(1),\ldots,{z}_{j}(M)\right)
%\end{align}
%with 
%\begin{align}
%{\phi}_{jli}(m) = \frac{\big({r}_{jli}(m)\big)^{2}}{\sum\limits_{n=1}^{L} {r}_{jni}(m) + \frac{1}{\rho^{\rm{tr}}}}
%\end{align}
\begin{align}\label{zjm}
{z}_{j}(m) = \sum\limits_{l=1}^{L} \sum\limits_{i=1}^{K} ({r}_{jli}(m) - {\phi}_{jli}(m)) + \frac{1}{{\rho}}
\end{align}
and
      \begin{align}
{\Theta}_{jll'i}(m) = \frac{{r}_{jli}(m){r}_{jl'i}(m)}{\sum\limits_{n=1}^{L} {r}_{jni}(m) + \frac{1}{\rho^{\rm{tr}}}} = {\phi}_{jli}(m)\frac{{r}_{jl'i}(m)}{{r}_{jli}(m)}.
  \end{align}
Therefore, we have that 
    \begin{align}
\mu_{jlk} = \frac{1}{M} \sum\limits_{m=1}^{M}\frac{{\phi}_{jlk}(m)}{\frac{1}{M}\sum\limits_{l'=1}^{L}\sum\limits_{i=1}^{K}\frac{{\phi}_{jl'i}(m) }{1 + \mu_{jl'i}} + \frac{1}{M}{z}_j(m)}.
  \end{align}
  Solving with respect to $\{\mu_{jlk}\}$ yields
      \begin{align}
\mu_{jlk}^\star =  \frac{1}{M}\sum\limits_{m=1}^{M} \frac{{\phi}_{jlk}(m)}{\varsigma_{j}^\star(m)}
  \end{align}
  with $\varsigma_{j}^\star(m)$ given by \eqref{varsigma_j} (where we have used \eqref{zjm}). If two cells are active, we have that
\begin{align}\label{SNR_two_cell}
\overline{\gamma}_{1k}^{\rm {ul}} = \big[\vect{Z}_{1k} \big]_{1,1} - \frac{\big[\vect{Z}_{1k} \big]_{1,2}\big[\vect{Z}_{1k} \big]_{2,1}}{1+ \big[\vect{Z}_{1k} \big]_{2,2}}
\end{align}
with $\big[\vect{Z}_{1k} \big]_{l,l'}=\frac{1}{M}\sum\limits_{m=1}^{M} \frac{{\phi}_{1lk}(m)}{\varsigma_1^\star(m)} \frac{{\beta}_{1l'k}(m)}{{\beta}_{1lk}(m)}$. Putting all the results together yields \eqref{gamma_diagonal}.
  
  \section*{Appendix D}
Following \cite[Sec.~IV]{Hoydis2013}, we assume that
   \begin{align}\label{sigma_jk}
{\bf H}_{jj} = {\bf A}{\bf V}_{jj} \quad {\bf H}_{jl} = \sqrt{\alpha}{\bf A}{\bf V}_{jl}
  \end{align}
  where ${\bf A}\in\mathbb{C}^{M\times M}$ is an arbitrary unitary matrix $M\times M$ matrix, ${\bf V}_{jj}\in\mathbb{C}^{M\times K}$ are standard
complex Gaussian matrices and $\alpha \in (0,1]$ is an intercell
interference factor. This implies that
 \begin{align}
\vect{\Phi}_{jlli} = \begin{cases}
 \nu{\bf I}_M & {\textrm{if }} j=l  \\ \\ 
\alpha \nu {\bf I}_M & {\textrm{if }} j\ne l
\end{cases}
\end{align}
with $\nu = \frac{{\rho^{\rm{tr}}}}{1+{\rho^{\rm{tr}}}\overline L}$ with $\overline L = 1 + \alpha(L-1)$. Also, we have that
   \begin{align}
\vect{Z}_{j}  = \Big(\frac{K}{M} (1-\nu)\overline L + \frac{1}{M\rho}\Big){\bf I}_M.
\end{align}
By using the above results, we obtain
 \begin{align}
 {\bf T}_{j}^{\star} =\left(\frac{K}{M}\overline L\eta^\star {\bf I}_M + \frac{1}{M{\rho}}{\bf I}_M\right)^{-1}
  \end{align}
  where
   \begin{align}
 \eta^\star =  \frac{1}{\overline L}\left(\frac{\nu}{1+\mu^\star} + \frac{\nu\alpha(L-1)}{1+\alpha\mu^\star}\right)+ (1-\nu)
   \end{align}
   with $\mu^\star$ being the solution of the set of fixed point equations. The latter can be computed with standard calculus, but it is not required for the subsequent analysis.
By using the above results, we have that 
 \begin{align}  \notag
 &  \big[\vect{Z}_{1k} \big]_{1,1} = \frac{1}{M}\tr \left(  \vect{\Phi}_{11k} {\bf T}_{1}^{\star}\right) \\\notag&=\frac{\nu}{M}\tr \left(  \left(\frac{K}{M}\overline L\eta^\star {\bf I}_M + \frac{1}{M{\rho}}{\bf I}_M\right)^{-1}\right)\\\notag&=\nu\left(\frac{K}{M}\overline L\eta^\star + \frac{1}{M{\rho}}\right)^{-1}\\&=\frac{\nu M}{{K\overline L\eta^\star}+\frac{1}{{\rho}}}\triangleq X.
   \end{align}
Assume for simplicity that $L=2$. By using similar steps as for $\big[\vect{Z}_{1k} \big]_{1,1}$, we obtain 
   \begin{align}
{\bf I}_2+ \vect{Z}_{1k}  = 
  \left[ {\begin{array}{cc}
   1+X & \alpha X \\
   \alpha X & 1+\alpha^2 X \\
  \end{array} } \right]
   \end{align}
such that \eqref{SNR_two_cell} reduces to
%    \begin{align}\label{sigma_jk}
%\big[\vect{Z}_{jk} \big]_{l,l'}= \begin{cases}
%\nu\frac{M}{K}\eta^\star& {\textrm{if }} l=l'  \\ \\ 
%\alpha^2\nu\frac{M}{K}\eta^\star & {\textrm{if }} l\ne l'
%\end{cases}
%\end{align}
\begin{align}\notag
\overline{\gamma}_{1k}^{\rm {ul}} &=X - \frac{(\alpha X)^2}{1+\alpha^2 X}=\frac{1}{X^{-1}+\alpha^2} \\
&= \frac{1}{\underbrace{\frac{1}{M{\rho}\nu}}_{\text{Noise}}+\underbrace{\frac{K}{M}\frac{\overline L}{\nu}\eta^\star}_{\text{Non-coherent Interference}}+\underbrace{\alpha(\overline L-1)}_{\text{Coherent interference}}}.
\end{align}
The above result is in a similar form of  \cite[Eq. (30)]{Hoydis2013}.
